# Supplementary material for: Strange metal behavior from incoherent carriers scattered by local moments
Source: arXiv:2306.12496 ancillary file (2023-07-11)
Supplement: Supplementary file 1 [file Supplementary-Materials.pdf]

# Strange metal behavior from incoherent carriers scattered by local moments. Supplementary Material

Sergio Ciuchi[1] and Simone Fratini[2]

[1] Dipartimento di Scienze Fisiche e Chimiche, Universitá dell'Aquila, Coppito-L'Aquila, Italy
[2] Université Grenoble Alpes, CNRS, Grenoble INP, Institut Néel, 38000 Grenoble, France

## I. DERIVATION OF THE DMFT RECURSION SCHEME

The action shown in Eqs. (1,2,3) can be derived by the following Hamiltonian within single site DMFT [1]

$$\begin{aligned} H &= -t \sum_{<i,j>,\sigma} c^{\dagger}_{i,\sigma} c_{j,\sigma} \\ &+ \sum_{i,\sigma,\rho} \sum_{\nu=0}^{3} g_{\nu} c^{\dagger}_{i,\sigma} \boldsymbol{\sigma}^{\nu}_{\sigma,\rho} c_{j,\rho} X^{\nu}_{i} \\ &+ \frac{1}{2} \sum_{\nu} k_{\nu} (X^{\nu}_{i})^2, \end{aligned} \tag{S.1}$$

where $c^{\dagger}_{i,\sigma}$ are creation operator of electrons at site $i$ and spin-component $\sigma$, $\boldsymbol{\sigma}^{\nu}$ are the Pauli matrices with $\nu = 0,3$ ($\boldsymbol{\sigma}^0 = 1$) and $X^{\nu}_i$ are the classical boson displacement operators. Electrons can hop with hopping integral $t$ and interact with the classical bosons through their charge ($\nu = 0$) and spin ($\nu > 0$).

The impurity propagator can be derived by averaging the matrix

$$\hat{G}(\omega) = \frac{1}{G_0^{-1}(\omega) - \sum_{\nu=0}^{3} g_{\nu} \boldsymbol{\sigma}^{\nu}_{\sigma,\rho} X^{\nu}} \tag{S.2}$$

over the classical phonon bath. The classical distribution functions for the bosons can be derived by integrating out the Gaussian electronic degree of freedom using the action Eqs. (1,2,3) of the main text

$$P(X^{\nu}) \propto \exp(-S_b)\ \Pi_n \det \left( G_0^{-1}(i\omega_n) \mathbf{1} - \sum_{\nu=0}^{3} g_{\nu} \boldsymbol{\sigma}^{\nu} X^{\nu} \right). \tag{S.3}$$

In the non ordered phase the impurity propagator obtained by averaging the matrix Eq. (S.2) with probability distribution Eq. (S.3) is spin independent and equal to

$$G(\omega) = \left\langle \frac{G_0^{-1}(\omega) + g_0 X^0 + \vec{v}(X^{\nu}) \cdot \boldsymbol{\sigma}}{(G_0^{-1}(\omega) - g_0 X^0)^2 - |\vec{v}(X^{\nu})|^2} \right\rangle, \tag{S.4}$$

where $\vec{v}$ is a three dimensional vector of components $v^{\nu} = g_{\nu} X^{\nu}$ ($\nu = 1,3$). The average over the classical boson variables restores translational invariance. The self-consistency condition is obtained by equating the impurity propagator with the local lattice propagator. Taking into account that in the paramagnetic case the self-energy is spin-independent we can write $G(\omega) = G_0^{-1}(\omega) - \Sigma(\omega)$ and

$$G(\omega) = \int d\epsilon N(\epsilon) \frac{1}{\omega + \mu - \epsilon - \Sigma(\omega)}, \tag{S.5}$$

where $N(\epsilon)$ is the non-interacting density of states (DOS) and $\mu$ the chemical potential.

In the DMFT calculation of the optical conductivity via the Kubo formula vertex corrections are absent. In the paramagnetic charge disordered case we obtain the usual expression [1]

$$\begin{aligned} Re\sigma(\omega) &= 2\bar{\sigma}\pi \int d\epsilon \int d\nu \Phi(\epsilon) A(\epsilon,\nu) A(\epsilon,\omega+\nu) \\ &\times \frac{f(\nu) - f(\omega+\nu)}{\omega}, \end{aligned} \tag{S.6}$$

where $A(\epsilon,\nu) = -Im\frac{1}{\pi}(\omega + \mu - \epsilon - \Sigma(\omega))^{-1}$ is the spectral function, $\Phi(\epsilon) = \sum_k |v_k|^2 \delta(\epsilon - \epsilon_k)$ is the transport function in a given direction ($v_k = \partial\epsilon(k)/\partial k$), $f(\nu)$ is the Fermi function and $\bar{\sigma} = e^2 a^2/\Omega\hbar/$ is the unit of conductivity with $a$ the lattice spacing in the chosen direction and $\Omega$ the volume of the unit cell. The DC conductivity is readily obtained as the zero frequency limit of the expression above,

$$\sigma(T) = 2\bar{\sigma}\pi \int d\epsilon \Phi(\epsilon) \int d\omega A^2(\omega,\epsilon) \left( -\frac{df}{d\omega} \right). \tag{S.7}$$

We consider an isotropic spin coupling preserving SU(2) symmetry ($g_{\nu} \equiv g_s$ for $\nu = 1,3$) and half filling ($\mu = 0$). In this case the distribution of the bosonic fields depends only on two variables: $X^0$, coupled to the charge, and the modulus of the boson displacement coupled to the spin, $r = \sqrt{\sum_{\nu=1}^{3} (X^{\nu})^2}$. Integrating out the electrons gives

$$\begin{aligned} P(X^0, r) &\propto \exp(-\frac{\beta}{2}(k_0 (X^0)^2 + k_s r^2)) \\ &\times \Pi_{n>0} \left| G_0^{-1}(i\omega_n) - g_0 X^0 - g_s r \right|^2 \\ &\times \left| G_0^{-1}(i\omega_n) - g_0 X^0 + g_s r \right|^2 \end{aligned} \tag{S.8}$$

where we have used the fact that $G_0^{-1}(-i\omega_n) = (G_0^{-1}(i\omega_n))^*$.

This probability distribution is even in the variable $X^0$ and depends on the variables coupled to the spin only through the modulus $r$. The averages appearing in in Eq. (S.4) therefore simplify to

$$G(\omega) = \left\langle \frac{G_0^{-1}(\omega)}{(G_0^{-1}(\omega) - g_0 X^0)^2 - g_s^2 r^2} \right\rangle, \tag{S.9}$$

where we have defines the average appearing in Eq. (S.9) as

$$\langle(...)\rangle = 4\pi \int dX_0 \int drr^2\,(...)$$

Two dimensionless coupling constants can be defined in this problem: the charge coupling $\lambda_c = g_0^2/2k_0D$ and the spin coupling $\lambda_s = g_s^2/2k_sD$. Accordingly we introduce two energy variables $u = g_0X^0$ and $v = g_sr$. Since from Eq. (S.8) $P(X^0, r) = P(X^0, -r)$ we can redefine the probability distribution of $v$ by extending it to both positive and negative values of $v$ as

$$\begin{aligned}\mathcal{P}(u,v) &\propto \exp(-(\frac{u^2}{4\lambda_c DT} + \frac{v^2}{4\lambda_s DT})) \\ &\times \Pi_{n>0}\left|G_0^{-1}(i\omega_n) - u - v\right|^2 \\ &\times \left|G_0^{-1}(i\omega_n) - u + v\right|^2. \end{aligned} \tag{S.10}$$

Eq. (S.9) can now be rewritten in a more compact form as

$$G(\omega) = \left\langle \frac{1}{G_0^{-1}(\omega) - u - v} \right\rangle \tag{S.11}$$

where the average is taken on the two-variable distribution $(4\pi v^2)\mathcal{P}(u,v)$.

All calculations presented here are performed on a Bethe lattice with an infinite coordination number $z \to \infty$ and half-bandwidth $D = \sqrt{z}t$, taking $D$ as the energy unit. The corresponding DOS and transport function appearing in Eqs. (S.5,S.6) read [2]

$$N(\epsilon) = \frac{2}{\pi D^2}\sqrt{D^2 - \epsilon^2}, \tag{S.12}$$

$$\Phi(\epsilon) = \frac{2}{3\pi D^2}(D^2 - \epsilon^2)^{3/2}, \tag{S.13}$$

with $\int \Phi(\epsilon)d\epsilon = D^2/4$. On the Bethe lattice $G_0^{-1}(i\omega_n) = i\omega_n - \frac{D^2}{4}G(i\omega_n)$ is known analytically. Eqs. (S.11,S.8) form a set of closed equations for the local Green's function $G(i\omega_n)$ that can be easily solved numerically by recursion.

## II. RESISTIVITY AT THE MIR LIMIT

By replacing $-df/d\omega = \delta(\omega - E_F)$ as appropriate at low temperatures and taking the weak scattering limit $\Gamma(E_F) = -2Im\Sigma(E_F) \ll D$, one obtains $\sigma = 2\bar{\sigma}\Phi(E_F)/\Gamma(E_F)$, cf. [3]. Observing that $2\bar{\sigma}\Phi(E_F) = ne^2/m$ for a parabolic dispersion in any dimensions recovers the Drude formula, $\sigma = ne^2\tau/m$, with $\tau = 1/\Gamma$.

Defining the Mott-Ioffe-Regel limit through the condition $k_F\ell = 1$ corresponds to $\Gamma = 2E_F$, yielding

$$\sigma_{MIR} = \bar{\sigma}\Phi(E_F)/E_F \tag{S.14}$$

on the parabolic band. This allows us to define $\rho_{MIR} = 1/\sigma_{MIR} = (3\pi/2)/\bar{\sigma}$ for the chosen semi-circular density of states, if we set $E_F = D$ at half filling. In these units, the low temperature limit of Eq. (S.7) acquires the simple expression

$$\rho/\rho_{MIR} = \Gamma/2D. \tag{S.15}$$

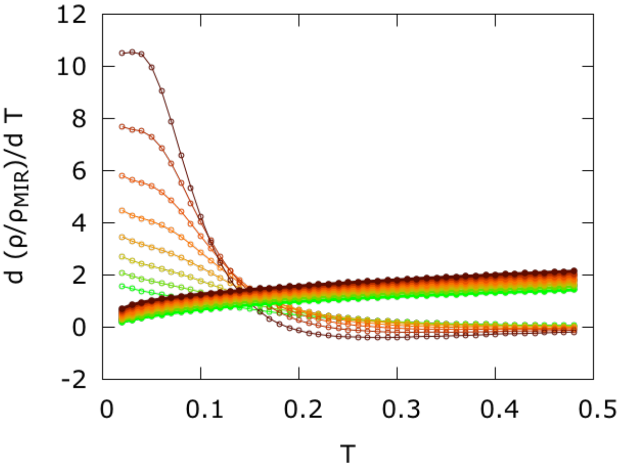


FIG. 1. The TCR of $\rho_\infty$ (closed symbols) and $\Delta\rho$ (open symbols) compared. The coupling ranges from $\lambda_s = 0.10$ (green) to $\lambda_s = 0.24$ (dark brown).

## III. THE INCOHERENT SCATTERING REGIME

In the incoherent scattering regime we start with the Kubo formula and implement the following high-temperature decoupling in the derivative of the Fermi function appearing in Eq. (4):

$$\left(-\frac{df}{d\omega}\right) = \frac{1}{4T}\left(1 - \tanh^2(\omega/2/T)\right). \tag{S.16}$$

Correspondingly the conductivity can be written as $\sigma = \sigma_\infty - \Delta\sigma$ where

$$\sigma_\infty(T) = 2\bar{\sigma}\pi\frac{1}{4T}\int d\epsilon\Phi(\epsilon)\int d\omega A^2(\epsilon,\omega). \tag{S.17}$$

By defining $\rho_\infty = 1/\sigma_\infty$ we can decouple the resistivity in a similar fashion as $\rho = \rho_\infty + \Delta\rho$. Fig. 1 shows that at high temperatures the variation with temperature of $\Delta\rho$ is negligible w.r.t. that of $\rho_\infty$.

We now evaluate the temperature coefficient of the resistivity (TCR, $B = d\rho/dT$) by considering the temperature variation of $\rho_\infty$. To provide an analytical estimate we take the incoherent approximation for the conductivity bubble,

$$\int d\epsilon\Phi(\epsilon)\int d\omega A^2(\epsilon,\omega) \simeq \frac{D^2}{4}\int d\omega A^2(\omega) \tag{S.18}$$

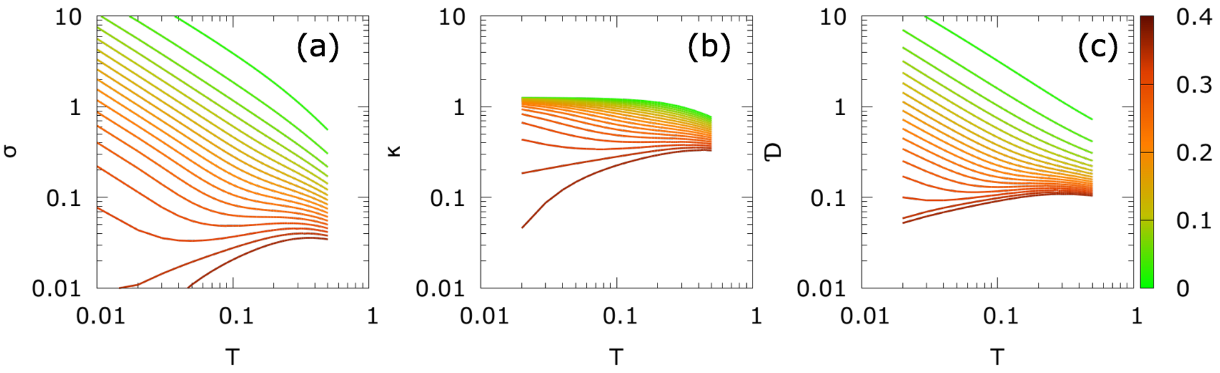


FIG. 2. (a) Conductivity, (b) Compressibility, (c) Diffusivity as a function of temperature for $\lambda_c = 0.0$ and $\lambda_s$ spanning from 0.0 to 0.4 (from green to red).

where $A(\omega)$ is the (momentum-integrated) spectral density. Within this approximation we obtain

$$d\rho_\infty/dT = \frac{8}{\pi\bar{\sigma}D^2 \int d\omega A^2(\omega)} \tag{S.19}$$

Using Eq. S.14 we can write more generally

$$\frac{d\rho_\infty/\rho_{MIR}}{d(T/D)} = C(T) \tag{S.20}$$

with $C(T)$ a *dimensionless* coefficient given by

$$C(T) = \frac{2\Phi(0)/\int \Phi(\epsilon)d\epsilon}{\pi \int d\omega A^2(\omega)} \tag{S.21}$$

for any lattice model and dimensionality.

The weak temperature dependence of this factor comes from the temperature dependence of the spectral function, due to interactions with the thermal bosons. In the classical limit the coupling with the bosons provides an effective disorder potential that broadens the original DOS [4]. Since $A(\omega)$ is normalized to one, the integral appearing in Eq. (S.21) is of the order of $1/D^*(T)$ where $D^* \simeq D\sqrt{1+8\lambda_s T/D}$ as can be estimated in the Gaussian limit [4], therefore providing only a moderate pre-asymptotic temperature dependence. The order of magnitude of $C$ can therefore be estimated using free-electron DOS: on the Bethe lattice $\Phi(0) = 2D/3\pi$, $\int \Phi(\epsilon)d\epsilon = D^2/4$ and the integral in Eq. (S.21) is $16/3\pi^2 D$, leading to $C = 1$.

The fact that the function $\Phi$, that embodies the specific properties of the lattice, appears both in the numerator and in the denominator of Eq. (S.21) makes this estimate quite robust. For example, repeating the same calculation for a box-like DOS mimicking the 2-dimensional lattice yields $C = 0.995$.

## IV. NERNST-EINSTEIN ANALYSIS

The Nerst-Einstein relation

$$\sigma = e^2\kappa\mathcal{D} \tag{S.22}$$

relates the conductivity $\sigma$ to the compressibility $\kappa$ and the diffusivity $\mathcal{D}$. In Eq. (S.22), $\sigma$ is known from the Kubo formula (Eq. (4), main text) whereas the compressibility can be derived by differentiating the particle number

$$n = \int d\nu f(\nu)A(\nu) \tag{S.23}$$

w.r.t. $\mu$. The diffusivity is obtained from these two quantities, via Eq. (S.22).

The temperature dependence of the quantities $\sigma$, $\kappa$ and $\mathcal{D}$ is shown in Fig. 2 for $\lambda_c = 0.0$, enabling a qualitative understanding of the different transport regimes. At weak coupling both diffusivity and compressibility are large and the temperature dependence of the conductivity is driven by the diffusivity [5, 6]. At strong coupling both the compressibility and the diffusivity are suppressed, leading to low-temperature insulating behaviour.

Interestingly, the strange metallic regime at high temperature and moderate $\lambda_s \simeq 0.2 - 0.3$ is characterized by a sizeable compressibility in comparison to the insulating phase, together with a suppressed diffusivity. The + and − sign in the legend of Fig. 2(e) of the main text indicate the qualitative amplitude of the components $\kappa$ and $\mathcal{D}$ in the different regimes of the phase diagram; the symbols +/− indicate sizable/suppressed values.

We note that in the strange metallic regime, the $1/T$ behavior of the conductivity cannot be ascribed individually to $\kappa$ or $\mathcal{D}$. Here the conductivity itself is the key quantity that carries the strange metal properties ($\rho \sim T$), while $\kappa$ and $\mathcal{D}$ show no obvious power law behavior.

Fig. 3 reports the $\lambda_s$-dependence of $\sigma$, $\kappa$ and $\mathcal{D}$ at a fixed temperature $T = 0.2$. At weak coupling the compressibility is close to one; the variation of $\sigma$ is dominantly driven by a reduction of the diffusivity with $\lambda_s$. Upon entering the strange metallic regime the reduction of conductivity results from a concomitant, yet weaker, decrease of both $\kappa$ and $\mathcal{D}$. Importantly, the diffusivity

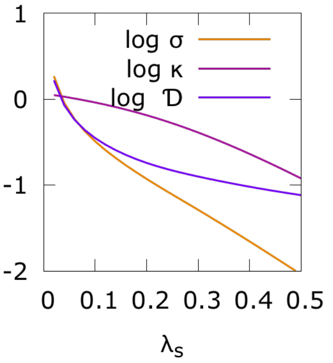


FIG. 3. Log of conductivity, compressibility and diffusivity as a function of $\lambda_s$ at $T = 0.2$. All quantities are expressed in units where $a = D = e = 1$

does not seem to saturate to any lower bound, in contradiction with recent proposals based on hydrodynamics [7].

## V. THE ATOMIC LIMIT, BOSON DISTRIBUTION AND LOCAL SPIN SUSCEPTIBILITY.

In the atomic limit $D \to 0$ we can rewrite the Hamiltonian as

$$H = H_b(X_0, r) + (g_0 X_0 - \mu)n + g\vec{\sigma} \cdot \vec{X} \quad \text{(S.24)}$$

where the boson part of the Hamiltonian is $H_b(X_0, r) = \frac{1}{2}k_0 X_0^2 + \frac{1}{2}kr^2$, $r^2 = \sum_{\nu=1}^{3} X_\nu^2$ and $n = n_\uparrow + n_\downarrow$. The half-filling condition is $\mu = \mu_0 = -g_0/k_0$. Upon shifting the chemical potential as $\mu' = \mu + g_0/k_0$ and the displacement coupled to the charge $X_0' = X_0 + g_0/k_0$, the four electronic states for any given value of classical displacements $X_\nu$ have the following energies:

$$|0\rangle \;:\; \Omega_0 = H_b(X_0', r) - g_0 X_0' \quad \text{(S.25)}$$
$$|+\rangle \;:\; \Omega_{1,+} = H_b(X_0', r) - \mu' + gr \quad \text{(S.26)}$$
$$|-\rangle \;:\; \Omega_{1,-} = H_b(X_0', r) - \mu' - gr \quad \text{(S.27)}$$
$$|\uparrow,\downarrow\rangle \;:\; \Omega_2 = H_b(X_0', r) - 2\mu' + g_0 X_0'. \quad \text{(S.28)}$$

(here $H_b(X_0', r)$ is the Gaussian part rewritten in term of the shifted $X_0'$).

By introducing the variables $u = g_0 X_0'$ and $v = gr$ the partition function reads

$$Z = \int du dv 4\pi v^2 e^{-\beta H_b} \left( e^{\beta u} + 2\cosh(\beta v) e^{\beta\mu'} + e^{\beta(2\mu' - u)} \right) \quad \text{(S.29)}$$

with $H_b = u^2/4\lambda_c D + v^2/4\lambda_s D$. We can now define a distribution function for the variables coupled to the spin ($v$) and to the charge ($u$), that we write at half-filling for sake of simplicity

$$4\pi v^2 \mathcal{P}(u, v) = \frac{4\pi v^2}{Z} \exp\left( -\frac{\beta u^2}{4\lambda_c D} - \frac{\beta v^2}{4\lambda_s D} \right) \times \times \; (\cosh(\beta u) + \cosh(\beta v)). \quad \text{(S.30)}$$

In the expression above, the Jacobian $4\pi v^2$ accounts for the the $SU(2)$ nature of the spin fluctuations, and $v$ extends to the whole $-\infty, \infty$ range. The $\cosh \beta u$ term in Eq. (S.30) is the contribution from empty and doubly occupied sites. When multiplied by the exponential prefactor it gives rise to two Gaussians in the variable $u$ peaked around $u_0 = \pm 2\lambda_c D$. The term proportional to $\cosh \beta v$ comes from the singly occupied sites and and again gives rise to two Gaussians in the variable $v$, peaked around $v_0 = \pm 2\lambda_s D$. In the case of a pure spin coupling only three Gaussian contributions remain in the variable $v$: one peaked around $v = 0$ coming from doubly occupied and empty sites, and two peaks at symmetric values of $v = \pm v_0$ arising from singly occupied sites. The fitting procedure of Fig. 2(a) is based on this result.

When generalized to include both spin- and charge-coupled fields with displacements $v_0$,$u_0$ and general variances $\sigma_s^2$,$\sigma_c^2$ the distribution Eq. (S.30) reads

$$4\pi v^2 \mathcal{P}(u, v) = \frac{4\pi v^2}{Z} \exp(-\frac{u^2}{2\sigma_c^2} - \frac{v^2}{2\sigma_s^2}) \times \times \left( \cosh(\frac{u_0 u}{\sigma_c^2}) + \cosh(\frac{v_0 v}{\sigma_s^2}) \right). \quad \text{(S.31)}$$

Using the distribution Eq. (S.31) one can derive the following results

$$< v^2 > = 3\sigma_s^2 \frac{(x_0^4/3 + 2x_0^2 + 1)e^{\frac{x_0^2}{2}} + 1}{(x_0^2 + 1)e^{\frac{x_0^2}{2}} + 1} \quad \text{(S.32)}$$

$$< u^2 > = \sigma_c^2 \frac{(x_0^2 + 1)e^{\frac{x_0^2}{2}} + 1}{e^{\frac{x_0^2}{2}} + 1}, \quad \text{(S.33)}$$

valid respectively in the case of pure spin (Eq. (S.32)) and in the case of pure charge (Eq. (S.32)) couplings. In Eq. (S.32) $x_0 = v_0/\sigma_s$ and in Eq. (S.33) $x_0 = u_0/\sigma_c$. In the limit $x_0 \ll \sigma$ we obtain $s^2 \equiv< v^2 > /3 = \sigma_s^2 + v_0^2/2$ for $\lambda_c = 0$ as reported in the main text. For $\lambda_s = 0$ we have instead $< u^2 >= \sigma_c^2 + u_0^2$.

Using the general result derived in Ref. [8] we can relate the variance of the centroid distribution of Stratonovich-Hubbard bosons to the local spin (or charge) susceptibility. Using Eq. (9) of ref. [8] we have

$$\chi^{loc} = \frac{1}{2\lambda_\nu D} \left( \frac{< \Delta^2 X_\nu >}{< \Delta^2 X_\nu >_0} - 1 \right) \quad \text{(S.34)}$$

where $\chi^{loc}$ is the local susceptibility to an external field which couples to the charge ($\nu = 0$) or to the spin ($\nu = 1, 2, 3$), $\lambda_\nu$ is the coupling (spin or charge), $< \Delta^2 X_\nu >$ is the mean square displacement of the bosonic field

whereas $< \Delta^2 X_\nu >_0$ is the same evaluated in the non-interacting system.

In the limit $v_0^0 < \sigma_s^2$ Eqs. (S.32,S.34) the local spin susceptibility can be decomposed into $\chi^{loc} = \chi_0 + \Delta\chi$ where

$$\chi_0 = \frac{1}{2\lambda_s D}\frac{v_0^2}{2\sigma_0^2} \tag{S.35}$$

is the term associated to the local moments and $\sigma_0^2 = 2\lambda_s DT$. The contribution associated to fluctuations reads

$$\Delta\chi = \frac{1}{2\lambda_s D}\left(\frac{\sigma_s^2}{\sigma_0^2} - 1\right). \tag{S.36}$$

Notice that approaching the atomic limit Eq. (S.35) gives rise to the Curie $1/T$ behaviour for the local spin susceptibility.

## VI. SPECTRAL FUNCTION AND MIT

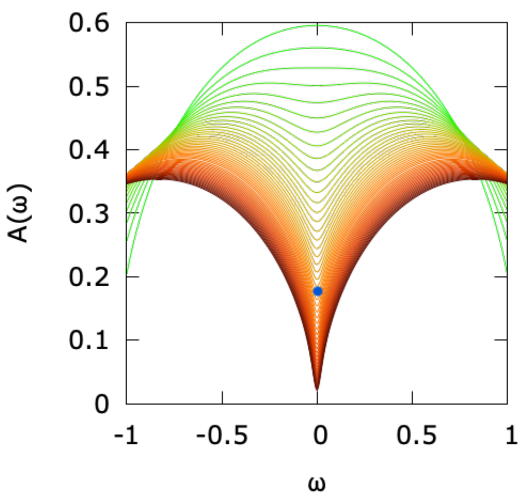


FIG. 4. Spectral function vs. temperature at $\lambda_s = 0.20$ and $\lambda_c = 0.00$; $T$ ranges from 0.02 to 0.50. The blue dot indicates the pseudogap value at $T = 0.25$.

Fig. 4 illustrates the opening of a pseudogap in the spectral function, for $\lambda_s = 0.20$ as a function of temperature. The blue dot marks the pseudogap value at the temperature $T = 0.25$ corresponding to the distribution $P$ depicted in Fig. 2(a). While the radial distribution of the spin variable $v$ does not show a well-defined peak, a pseudogap is formed in the spectral function as consequence of the $SU(2)$ nature of the spin fluctuations, via the Jacobian $4\pi v^2$ that effectively splits the distribution into two separate peaks. In the local moment regime a pseudogap forms gradually in the spectral function upon increasing $\lambda_s$, eventually leading to a genuine MIT at $T = 0.0$ at a critical value of the spin coupling. The pseudogap also arises upon increasing $T$, without however inducing a MIT: at high temperatures the system behaves as a strange metal as described in the preceding Sections and in the main text.


[1] A. Georges, G. Kotliar, W. Krauth, and M. J. Rozenberg, Dynamical mean-field theory of strongly correlated fermion systems and the limit of infinite dimensions, Rev. Mod. Phys. **68**, 13 (1996).

[2] A. Chattopadhyay, A. J. Millis, and S. Das Sarma, Optical spectral weights and the ferromagnetic transition temperature of colossal-magnetoresistance manganites: Relevance of double exchange to real materials, Phys. Rev. B **61**, 10738 (2000).

[3] X. Deng, J. Mravlje, R. Žitko, M. Ferrero, G. Kotliar, and A. Georges, How bad metals turn good: Spectroscopic signatures of resilient quasiparticles, Phys. Rev. Lett. **110**, 086401 (2013).

[4] S. Fratini and S. Ciuchi, Spectral properties and isotope effect in strongly interacting systems: Mott-Hubbard insulator versus polaronic semiconductor, Phys. Rev. B **72**, 235107 (2005).

[5] J. Kokalj, Bad-metallic behavior of doped Mott insulators, Phys. Rev. B **95**, 041110(R) (2017).

[6] N. Pakhira and R. H. Mackenzie, Absence of a quantum limit to charge diffusion in bad metals, Phys. Rev. B **91**, 075124 (2015).

[7] S. A. Hartnoll, Theory of universal incoherent metallic transport, Nature Physics **11**, 54 (2015).
[8] S. Ciuchi, G. Sangiovanni, and M. Capone, Pairing and polarization in electron-boson systems with retarded interactions via dynamical mean-field theory, Phys. Rev. B **73**, 245114 (2006).
